# Supplementary material for: AoI-based Finite Horizon Scheduling for Heterogeneous Networked Control Systems
Source: arXiv:2005.02037 source file (2020-05-05)
Supplement: Supplementary file 1 [file appendix.tex]

\appendix
\subsection{Proof of probability mass functions for different number of hops}
\label{sec:appendic}
In this appendix we share the derivation of probability functions and the expectations.  For instance for the probability of occurrence of any age with 2 hops is
\begin{align}
\text{Pr}[\Delta_2(t)=\delta_2]= & \sum_{\delta_1=0}^{\delta_2} (1-p_1) \cdot {p_1}^{\delta_1} \cdot  (1-p_2) \cdot {p_2}^{\delta_2-\delta_1} \nonumber\\
%= & (1-p_1)(1-p_2){p_2}^{\delta_2}\sum_{\delta_1=0}^{\delta_2}  \cdot \left({\frac{p_1}{p_2}}\right) ^{\delta_1}\nonumber \\
= & (1-p_1)(1-p_2){p_2}^{\delta_2} \cdot \frac{1-\left({\frac{p_1}{p_2}}\right) ^{\delta_2+1}}{1-{\frac{p_1}{p_2}}}\nonumber \\ 
= & (1-p_1)(1-p_2)\cdot \frac{{p_2}^{\delta_2+1}-{p_1}^{\delta_2+1}}{{p_2}-{p_1}}.
\end{align}
%We simply make use of finite power sum calculation and do the further simplifications. For the expected age, we use our findings for a single occurrence and apply the expectation formula,
%\begin{align*}
%\E[\Delta_2] =& \sum_{\delta_2}^\infty \delta_2 (1-p_1)(1-p_2)\cdot \frac{{p_2}^{\delta_2+1}-{p_1}^{\delta_2+1}}{{p_2}-{p_1}} \nonumber\\
%%= & \frac{(1-p_1)(1-p_2)}{{p_2}-{p_1}}\left( \sum_{\delta}\delta_2{p_2}^{\delta_2+1} - \sum_{\delta}\delta_2{p_1}^{\delta_2+1}\right)\nonumber\\
%=& \frac{(1-p_1)(1-p_2)}{{p_2}-{p_1}} \left(\left( \frac{{p_2}}{1-p_2}\right)^2  -\left(\frac{p_1}{1-p_1}\right)^2   \right) \nonumber\\
%=& \frac{p_1}{1 - p_1} + \frac{p_2}{1 - p_2}.
%\end{align*}
For the 3-hop scenario, probability of an age $\delta_3$ can be obtained from Eq.~\eqref{eq:n_hop_age_1} by plugging in our results for $\Delta_2$:
\begin{align*}
\text{Pr}& [\Delta_3(t)=\delta_{3}] = \sum_{\delta_{2}=0}^{\delta_{3}}  (1-p_3){p_3}^{\delta_3-\delta_2} \nonumber \\ &\cdot (1-p_1)(1-p_2)\cdot \frac{{p_2}^{\delta_2+1}-{p_1}^{\delta_2+1}}{{p_2}-{p_1}}\nonumber \\
%& = \frac{{p_3}^{\delta_3+1}\prod^3_{i=1} (1-p_i)}{p_2-p_1} \nonumber \\ & \cdot \sum_{\delta_{2}=0}^{\delta_{3}}\left(\left(\frac{p_2}{p_3}\right)^{\delta_2+1} -\left(\frac{p_1}{p_3}\right)^{\delta_2+1}        \right)\nonumber \\
&= \frac{{p_3}^{\delta_3+1}\prod^3_{i=1} (1-p_i)}{p_2-p_1} \nonumber \\ & \cdot \left( \left(\dfrac{p_2}{p_3}\right)\frac{1-\left({\frac{p_2}{p_3}}\right) ^{\delta_3+1}}{1-{\frac{p_2}{p_3}}} -\left( \dfrac{p_1}{p_3} \right)\frac{1-\left({\frac{p_1}{p_3}}\right) ^{\delta_3+1}}{1-{\frac{p_1}{p_3}}} \right)\nonumber \\
%& = \frac{\prod^3_{i=1} (1-p_i)}{p_2-p_1} \nonumber \\ & \cdot \left( p_2 \cdot \frac{{p_3}^{\delta_3+1}-{p_2}^{\delta_3+1}} {{p_3}-{p_2}} -{p_1} \cdot \frac{{p_3}^{\delta_3+1}-{p_1}^{\delta_3+1}}{{p_3}-{p_1}} \right)
%\nonumber \\
&  = \frac{\prod^3_{i=1} (1-p_i)}{p_2-p_1} \cdot \sum_{j=1}^2 (-1)^j \cdot {p_j} \cdot \frac{{p_3}^{\delta_3+1}-{p_j}^{\delta_3+1}}{{p_3}-{p_j}} 
\end{align*}
